# Supplementary material for: Vertex Ordering for Exact Triangle Listing: Concave Geometry and Certified Rounding
Source: arXiv:2610.24314 source file (2026-10-16)
Supplement: Supplementary file 1 [file supp_heldout_rows.tex]

Email-Eu-core & Neigh3 & 6.51 & 3.22 & 3.17 & 3.26 & 3.50$\pm$0.01 \\
CollegeMsg & Neigh4-rev & 18.82 & 3.04 & 2.86 & 2.75 & 3.07$\pm$0.00 \\
LastFM-Asia & Neigh2 & 2.74 & 5.88 & 4.22 & 4.57 & 6.01$\pm$0.19 \\
Deezer-Europe & Neigh5 & 4.34 & 5.23 & 3.25 & 3.53 & 4.92$\pm$0.02 \\
Amazon0302 & Neigh1-rev & 6.18 & 2.72 & 0.39 & 0.00 & 2.39$\pm$0.05 \\
Wiki-Talk$^\dagger$ & Degree & 0.00 & 13.04 & 11.48 & 10.97 & 13.04$\pm$0.02 \\
com-Youtube & Neigh3-rev & 13.61 & 12.52 & 15.61 & 13.78 & 16.14$\pm$0.01 \\
web-Google & Neigh3-rev & 4.08 & 1.13 & 0.93 & 0.00 & 1.39$\pm$0.00 \\
roadNet-CA & Neigh3-rev & 18.72 & 18.18 & 0.05 & 0.00 & 17.07$\pm$0.00 \\
\midrule
Mean & & 8.33 & 7.22 & 4.66 & 4.32 & 7.50 \\
